# Supplementary material for: Cognitive Modeling of Semantic Fluency Using Transformers
Source: arXiv:2208.09719 source file (2022-08-20)
Supplement: Supplementary file 1 [file appendix.tex]

\appendix

\section{Code and Runtime}
All the code for the experiments (will be released publicly upon paper acceptance) in this paper was run on a Ubuntu 18.04.4 server with 128GB RAM, 64 cores, and 3 NVIDIA Tesla V100-PCIE-32GB GPUs.

\section{Data Cleaning}
\label{sec:data_cleaning}
    The SNAFU Sample dataset comes with multiple issues that we needed to address in order to prepare the data for our experiments; issues like misspellings, such as `appl' instead of `apple', and multiple words joined together in the released version, such as `polarbear' instead of `polar bear', and their combinations. These words cause lower performance of our models, as they do not exist in the vocabulary of the models. We implemented a tool to clean the data, so that it can be used in our experiments without causing the performance drop. In particular, the following techniques were used to eliminate the errors:
    \begin{enumerate}
        \item{We first extracted words from the ConceptNet\footnote{\url{https://conceptnet.io/}} semantic network using the categories from the SNAFU dataset as ``concepts'' and filtered out only those which fall in the following relations with the category: `/r/AtLocation', `/r/DefinedAs', `/r/FormOf', `/r/InstanceOf', `/r/IsA', `/r/MannerOf', `/r/PartOf'. If the instance of a category in the raw SNAFU dataset appears in the extracted list of instances for this category from Conceptnet, we leave it unchanged. If there is no exact match, we find the word in Conceptnet that has the smallest Levenshtein distance with the word in question. This allows us to correct misspellings and joined words.}
        \item{We lemmatize plural words to avoid duplicate instances in fluency lists, such as `cat' and `cats'.}
        \item{As a multiple-word instance in Conceptnet is represented with underscores in place of spaces, in the next step, we replace underscores with spaces.}
    \end{enumerate}

\begin{table}
\centering
\footnotesize
\resizebox{0.4\textwidth}{!}{
\begin{tabular}{|c|c|c|}
     \hline
     Approach & $N$ & Run time (hrs) \\
     \hline
     Random Baseline & 1 & 0.017 \\
     Random Walk on USF & 1 & 0.034 \\
     RoBERTa Large & 56 & 20 \\
     ClusteRoBERTa & 9 & 5 \\
     GPT2 Large & 48 & 90 \\
     \hline
\end{tabular}
}
\caption{The run time of each approach across all $N$ functions and all 796 SFLs based on that approach when $\sim$80\% GPU utilization was done for these experiments.}
\label{tab:runtime}
\end{table}

\section{Implementations}
We use multiple Python libraries in our code, mainly:
\begin{itemize}
    \item Preprocessing: NLTK's (Natural Language ToolKit) list of stopwords is used to eliminate stopwords from model predictions. Since the prediction `dogs' is acceptable when the item is `dog' and vice-versa, we lemmatize the words in the SFL as well as the ones predicted by our approaches. We also consider only the predictions that are nouns since we expect the items in an SFL to be almost exclusively nouns (due to the category words given). NLTK's \texttt{WordNetLemmatizer} is used for performing lemmatization and all the synsets with the letter `n' in WordNet are considered for filtering nouns. 
    \item Word2Vec: We used the Gensim implementation of Word2Vec\footnote{\url{https://radimrehurek.com/gensim/models/word2vec.html}} which has a function \texttt{most\_similar} that returns a list of words most similar to a given list of words.
    \item Transformers: Huggingface implements a majority of the latest transformer models and we use its implementation of RoBERTa\footnote{\url{https://huggingface.co/transformers/model_doc/roberta.html}} and GPT-2.\footnote{\url{https://huggingface.co/transformers/model_doc/gpt2.html}} The masked language modeling task is implemented using the \texttt{FillMaskPipeline} from Huggingface.
\end{itemize}

\section{Supplementary Results}
\label{sec:supplementary_results}

% \todoAnimesh{histogram of frequencies with which functions were chosen by CA}

The main paper shows a performance comparison of RoBERTa-Large prompts and context sizes. A similar comparison for ClusteRoBERTa context sizes and feature sizes is shown in Table \ref{tab:clus} and one for GPT-2 context and temperature values is shown in Table \ref{tab:gpt2}.

    \begin{table}
    \centering
    \footnotesize
    % \resizebox{0.48\textwidth}{!}{
    \begin{tabular}{|c||c|c|c|}
        \hline
        $ct$ & 1 & 2 & 3 \\
        \hline
        1 & -12.1 & -12.1 & -12.1 \\
        3 & -12.1 & -12.1 & -12.1 \\
        5 & -12.1 & -12.0 & -12.0 \\
        \hline
        1 & 17.4 & 18.1 & 18.4 \\
        3 & 19.6 & 20.0 & 20.3 \\
        5 & 19.2 & 19.6 & 20.1 \\
        \hline
    \end{tabular}
    % }
    \caption{Average scaled log-likelihoods (top) and top-5 accuracy (\%) (bottom) of CR feature size (columns) and context size (rows) combinations.}
    \label{tab:clus}
    \end{table}
    
    \begin{table}
    \centering
    \footnotesize
    % \resizebox{0.48\textwidth}{!}{
    \begin{tabular}{|c||c|c|c|}
        \hline
        $ct$ & 0.7 & 0.8 & 0.9 \\
        \hline
        0 & 1.3 & 1.3 & 1.6 \\
        1 & 14.0 & 13.6 & 13.2 \\ 
        5 & 12.9 & 12.6 & 12.2 \\
        25 & 13.4 & 13.0 & 12.3 \\
        \hline
    \end{tabular}
    % }
    \caption{Average scaled log-likelihoods (top) and top-5 accuracy (\%) (bottom) of GPT-2 temperature (columns) and context size (rows) combinations.}
    \label{tab:gpt2}
    \end{table}

While going through an SFL, CA reviews its choice of function on each item of the list. Figure \ref{fig:ca-switches} shows the percentage of times it actually changes its choice in relation to the window size CA works with.

\begin{figure}
    \centering
    \includegraphics[width=0.48\textwidth]{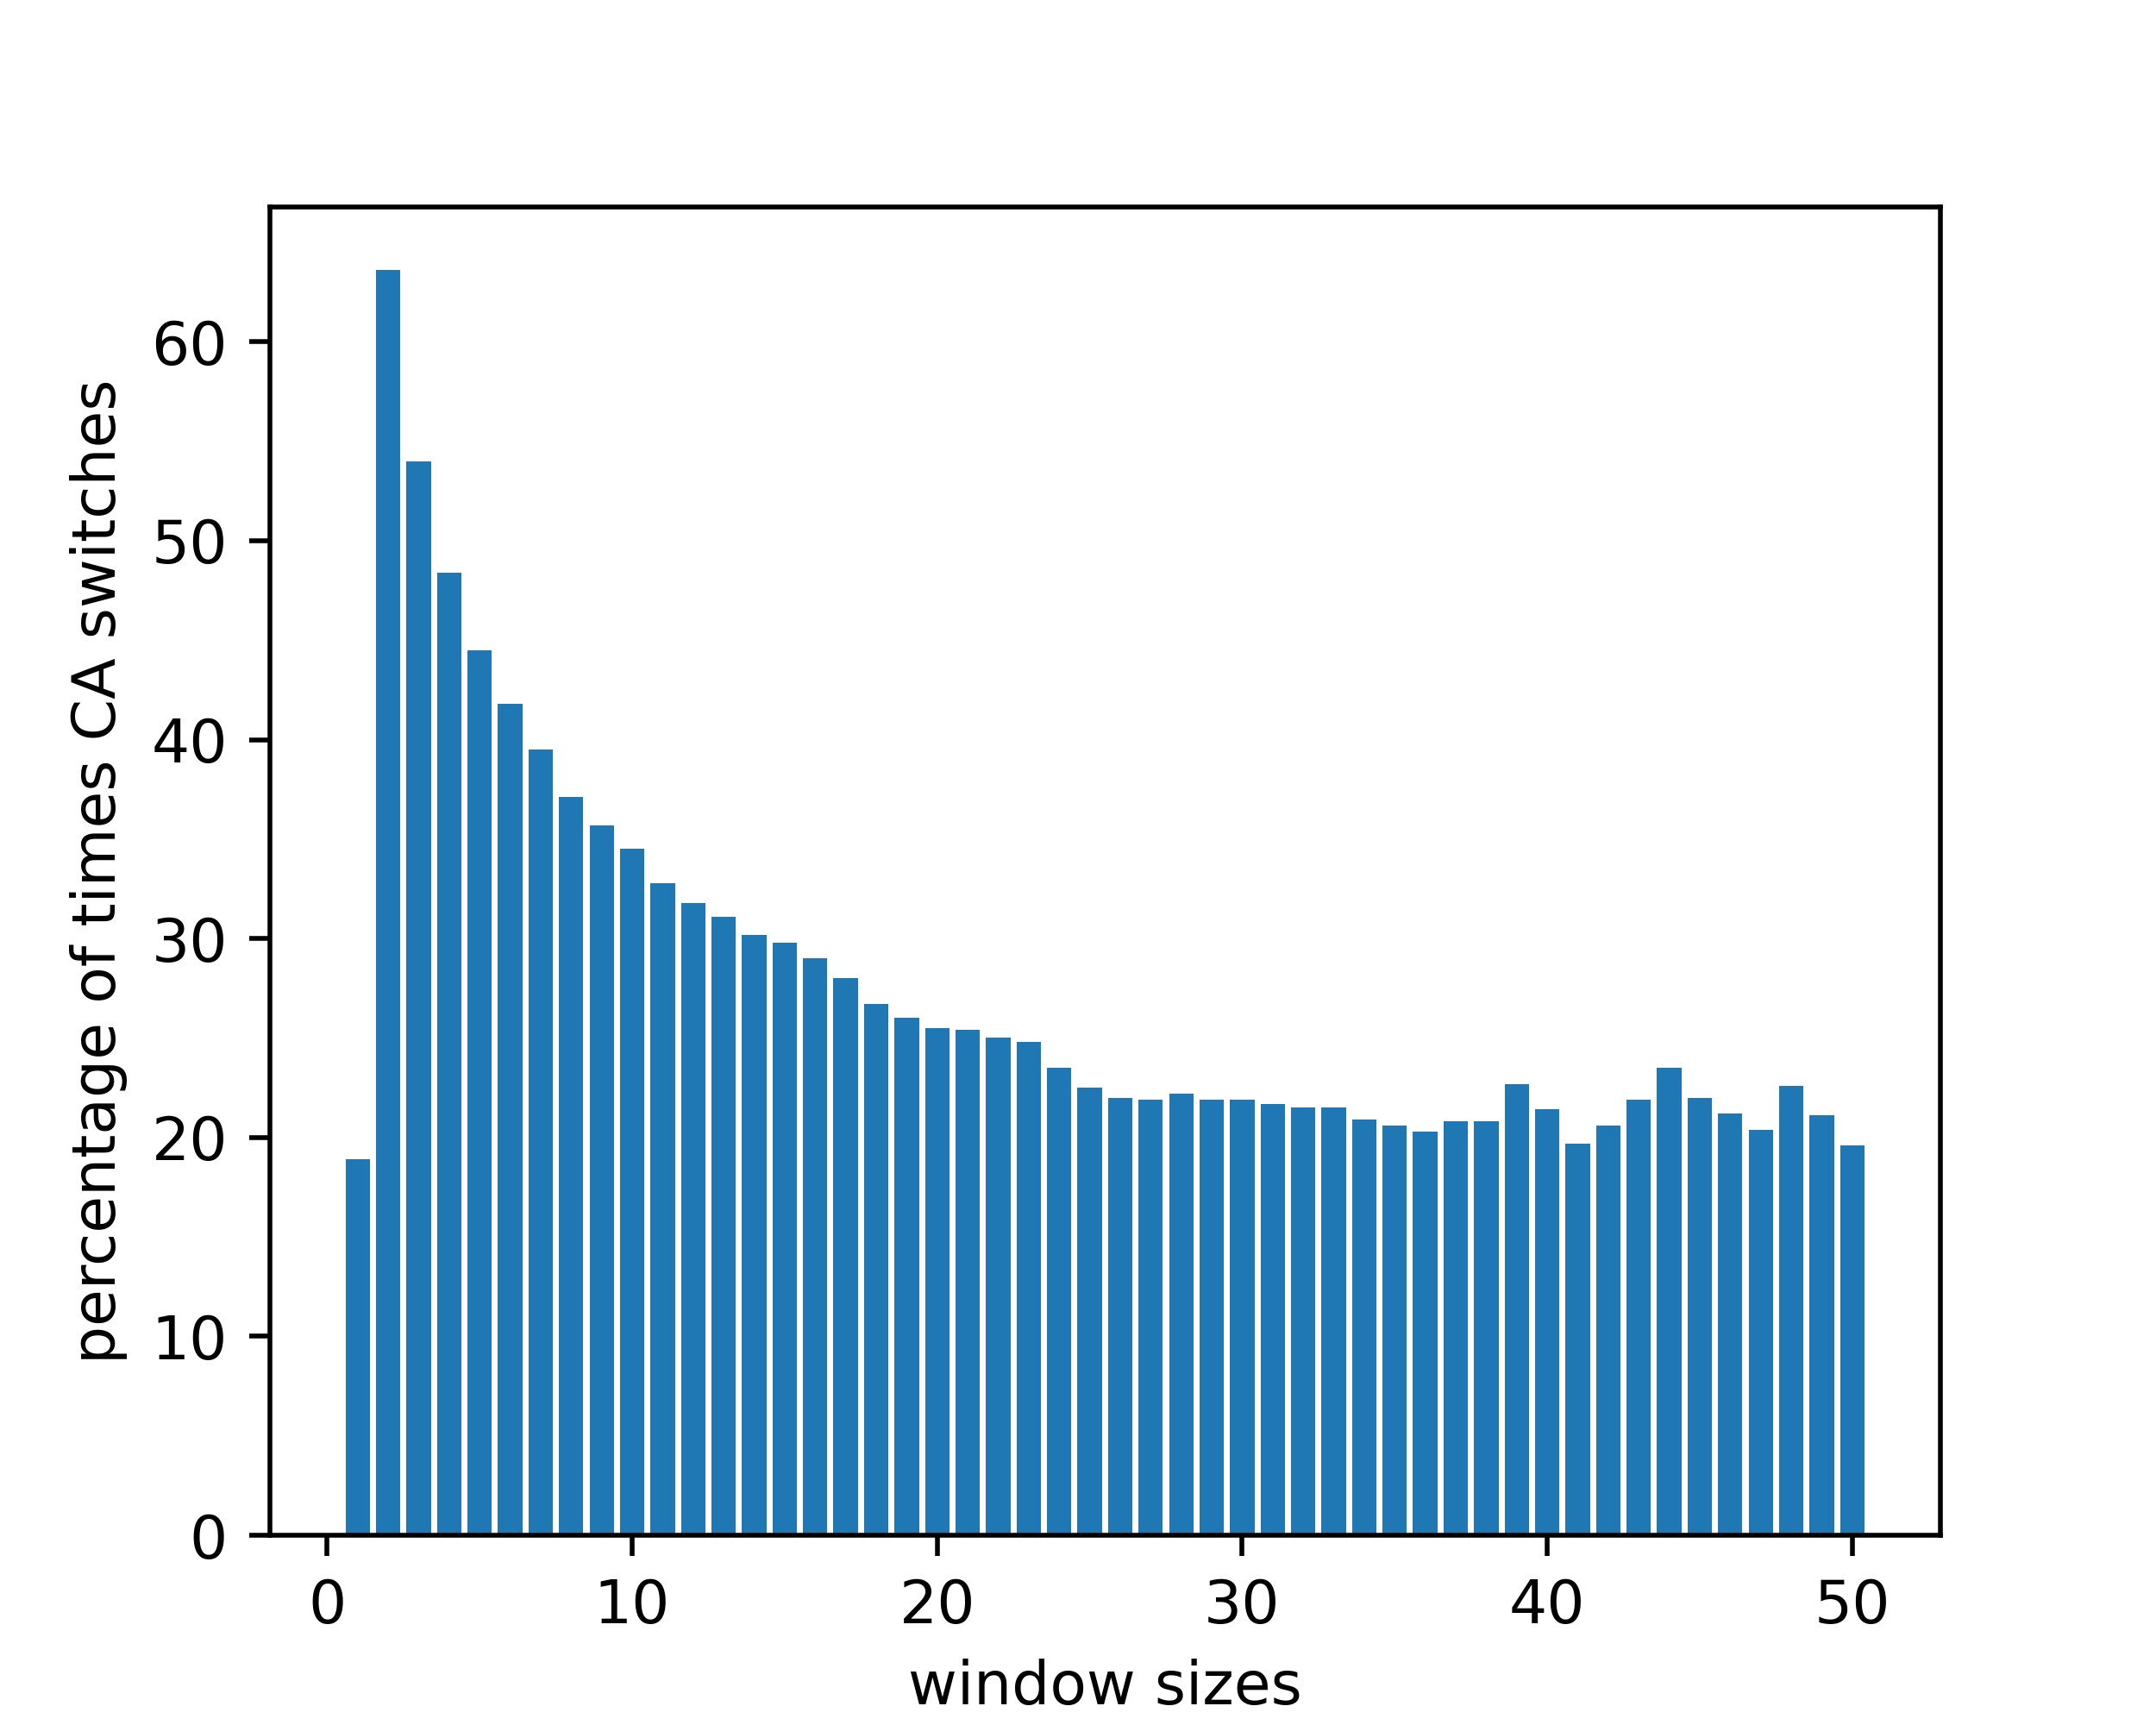}
    \caption{Percentage of times CA switches its choice for all window sizes between 1 and 50.}
    \label{fig:ca-switches}
\end{figure}

Though we show only the approaches' top-$5$ accuracy in the main paper, we plot the graphs for top-$1$ (Figure \ref{fig:top1}), top-$25$ (Figure \ref{fig:top25}), and top-$50$ (Figure \ref{fig:top50}) accuracies too. The point where ATC starts outperforming \textit{BI} is called ATC's \textit{$\textit{BI}$ crossover point}. We find that as $k$ increases, the crossover points shift towards the right (Table \ref{tab:crossovers}). It is evident that for higher values of $k$, the performance of static approaches starts improving and reaching close to optimal since the scoring criteria is not as strict anymore.
            \begin{table}
            \centering
            \footnotesize
            \begin{tabular}{|c||c|c|c|c|}
                 \hline
                 k & \multicolumn{2}{c|}{ATC crossover} & \multicolumn{2}{c|}{CA crossover} \\
                 \cline{2-5}
                 {} & $\textit{BO}$ & $\textit{BI}$ & $\textit{BO}$ & $\textit{BI}$ \\
                 \hline
                 1 & 5 & 10 & 7 & 12 \\
                 5 & 24 & 37 & 24 & 37 \\
                 25 & 37 & - & 37 & - \\
                 50 & 41 & - & 41 & - \\
                 \hline
            \end{tabular}
            % }
            \caption{Crossover points for ATC and CA.}
            \label{tab:crossovers}
            \end{table}

\begin{figure}
    \centering
    \includegraphics[width=0.48\textwidth]{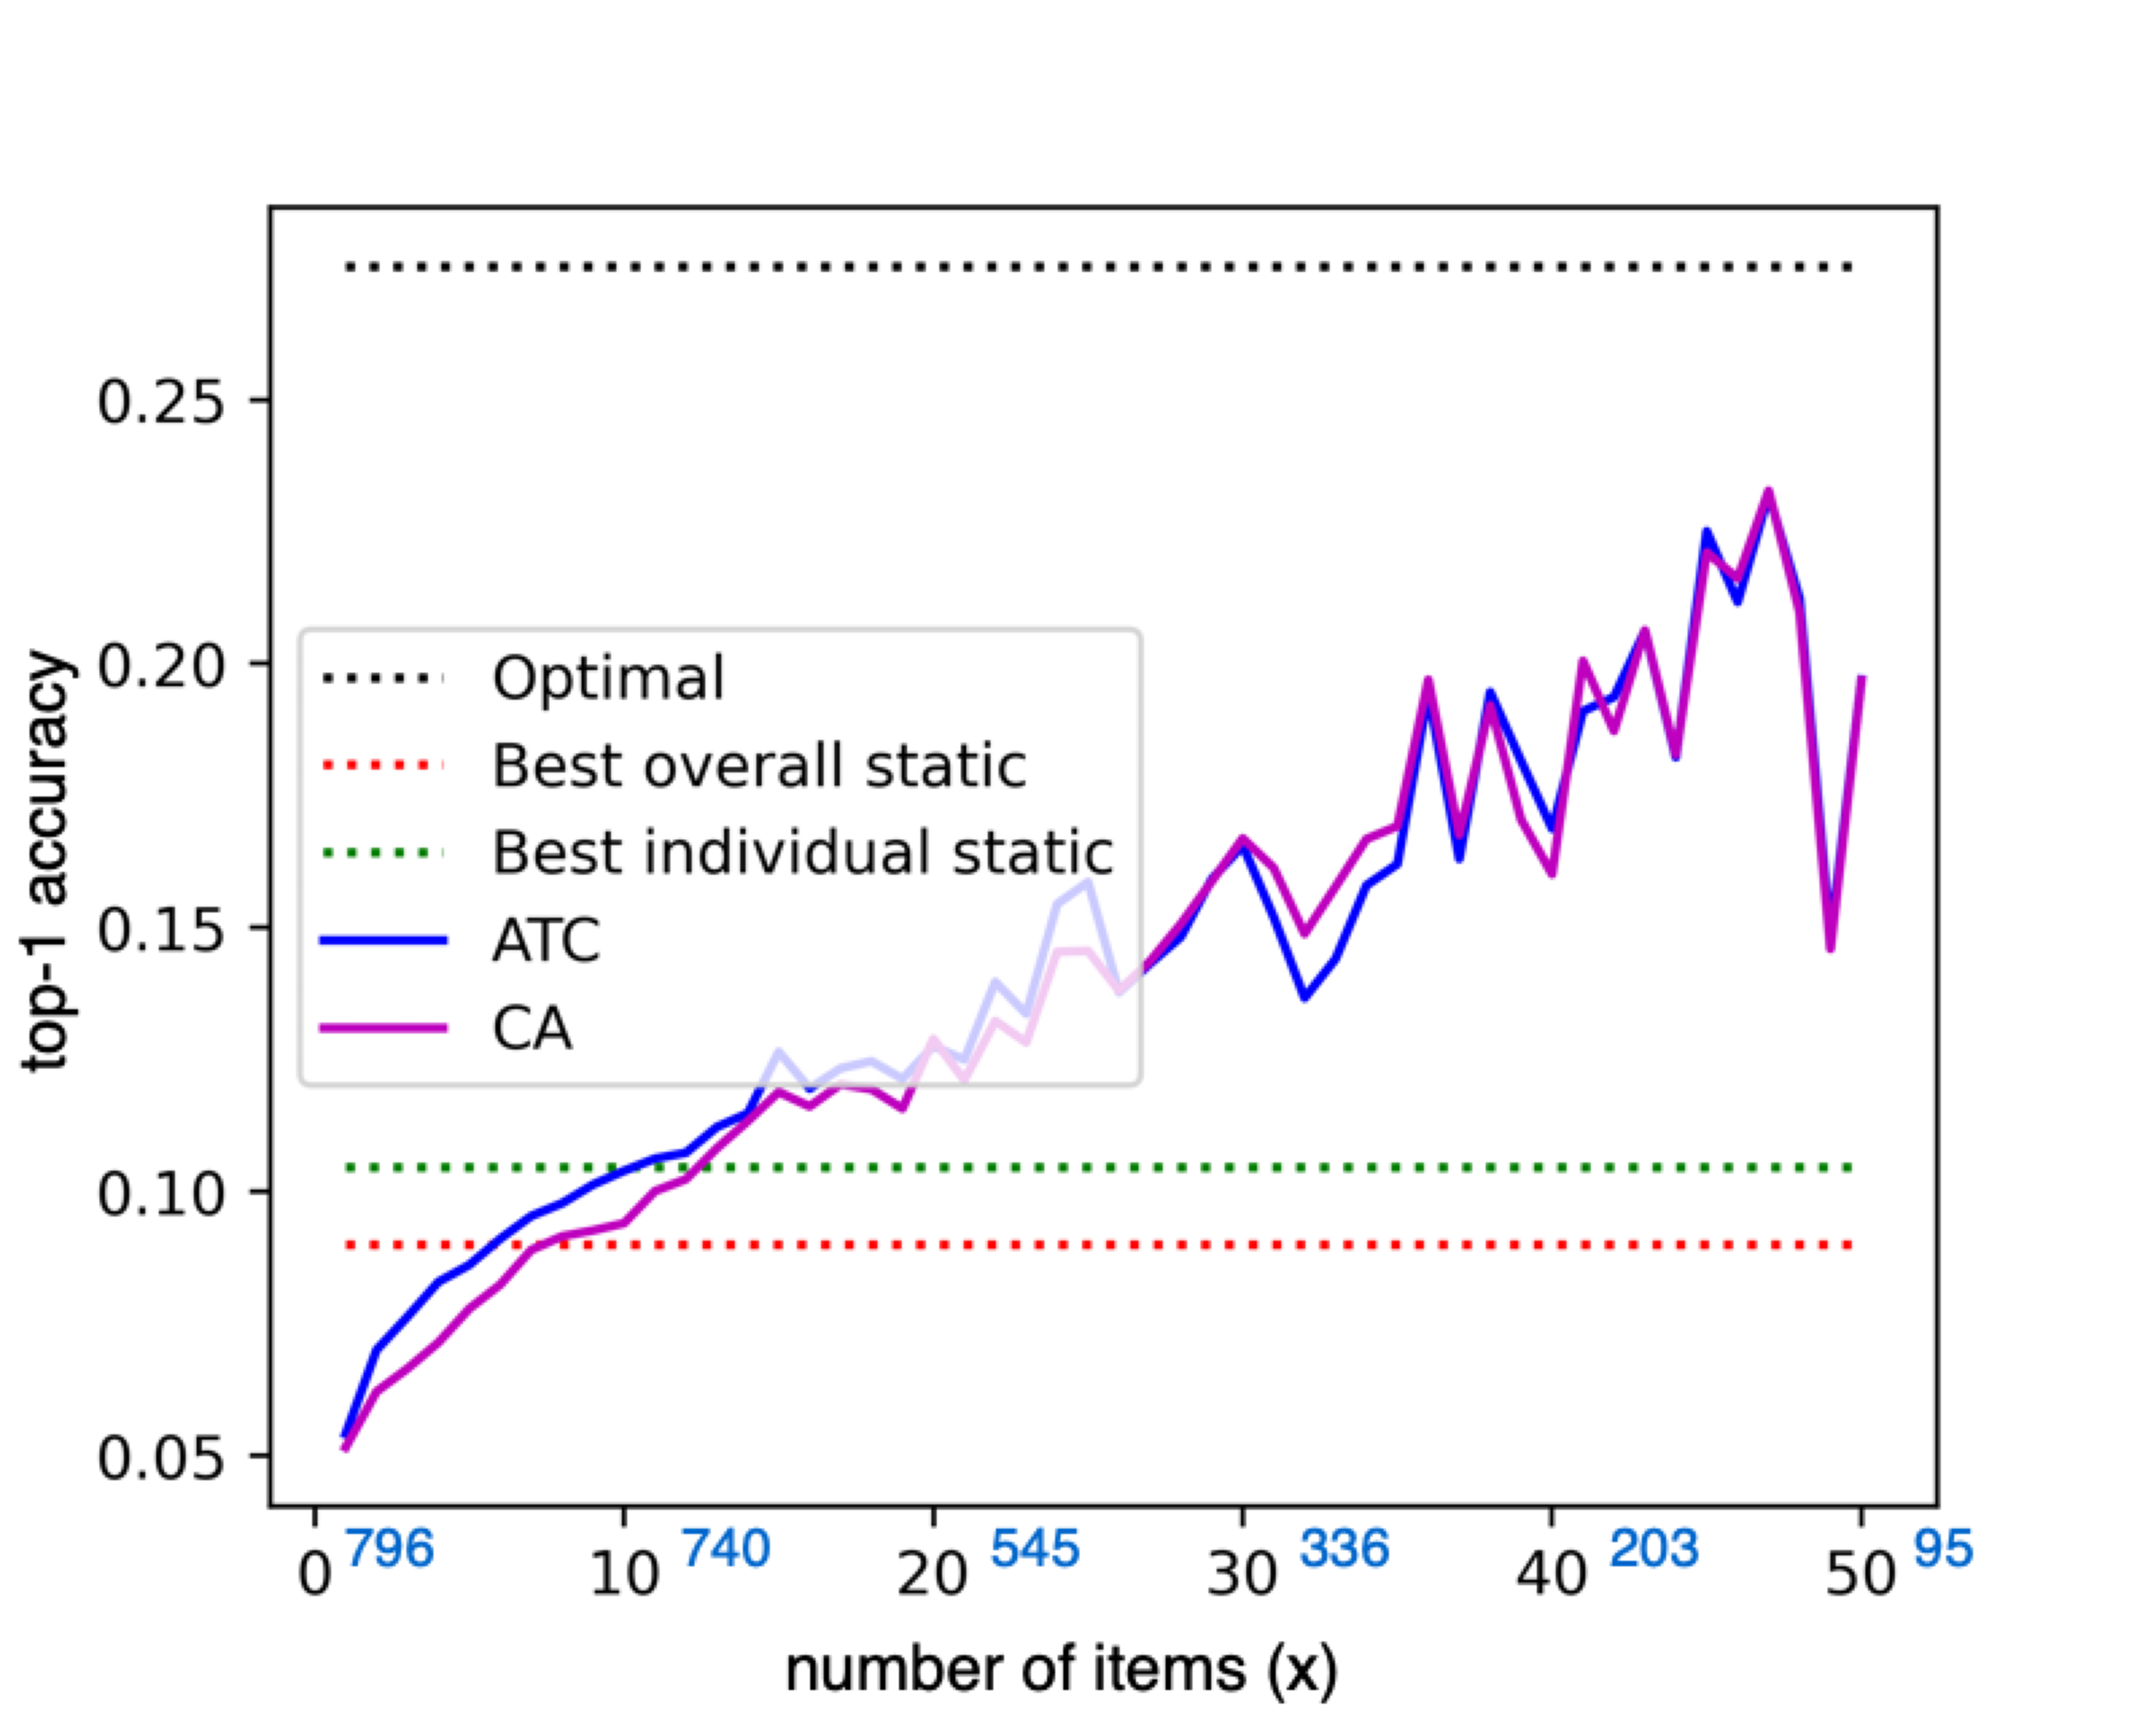}
    \caption{Top-$1$ accuracy comparison of adaptive and static approaches.}
    \label{fig:top1}
\end{figure}
\begin{figure}
    \centering
    \includegraphics[width=0.48\textwidth]{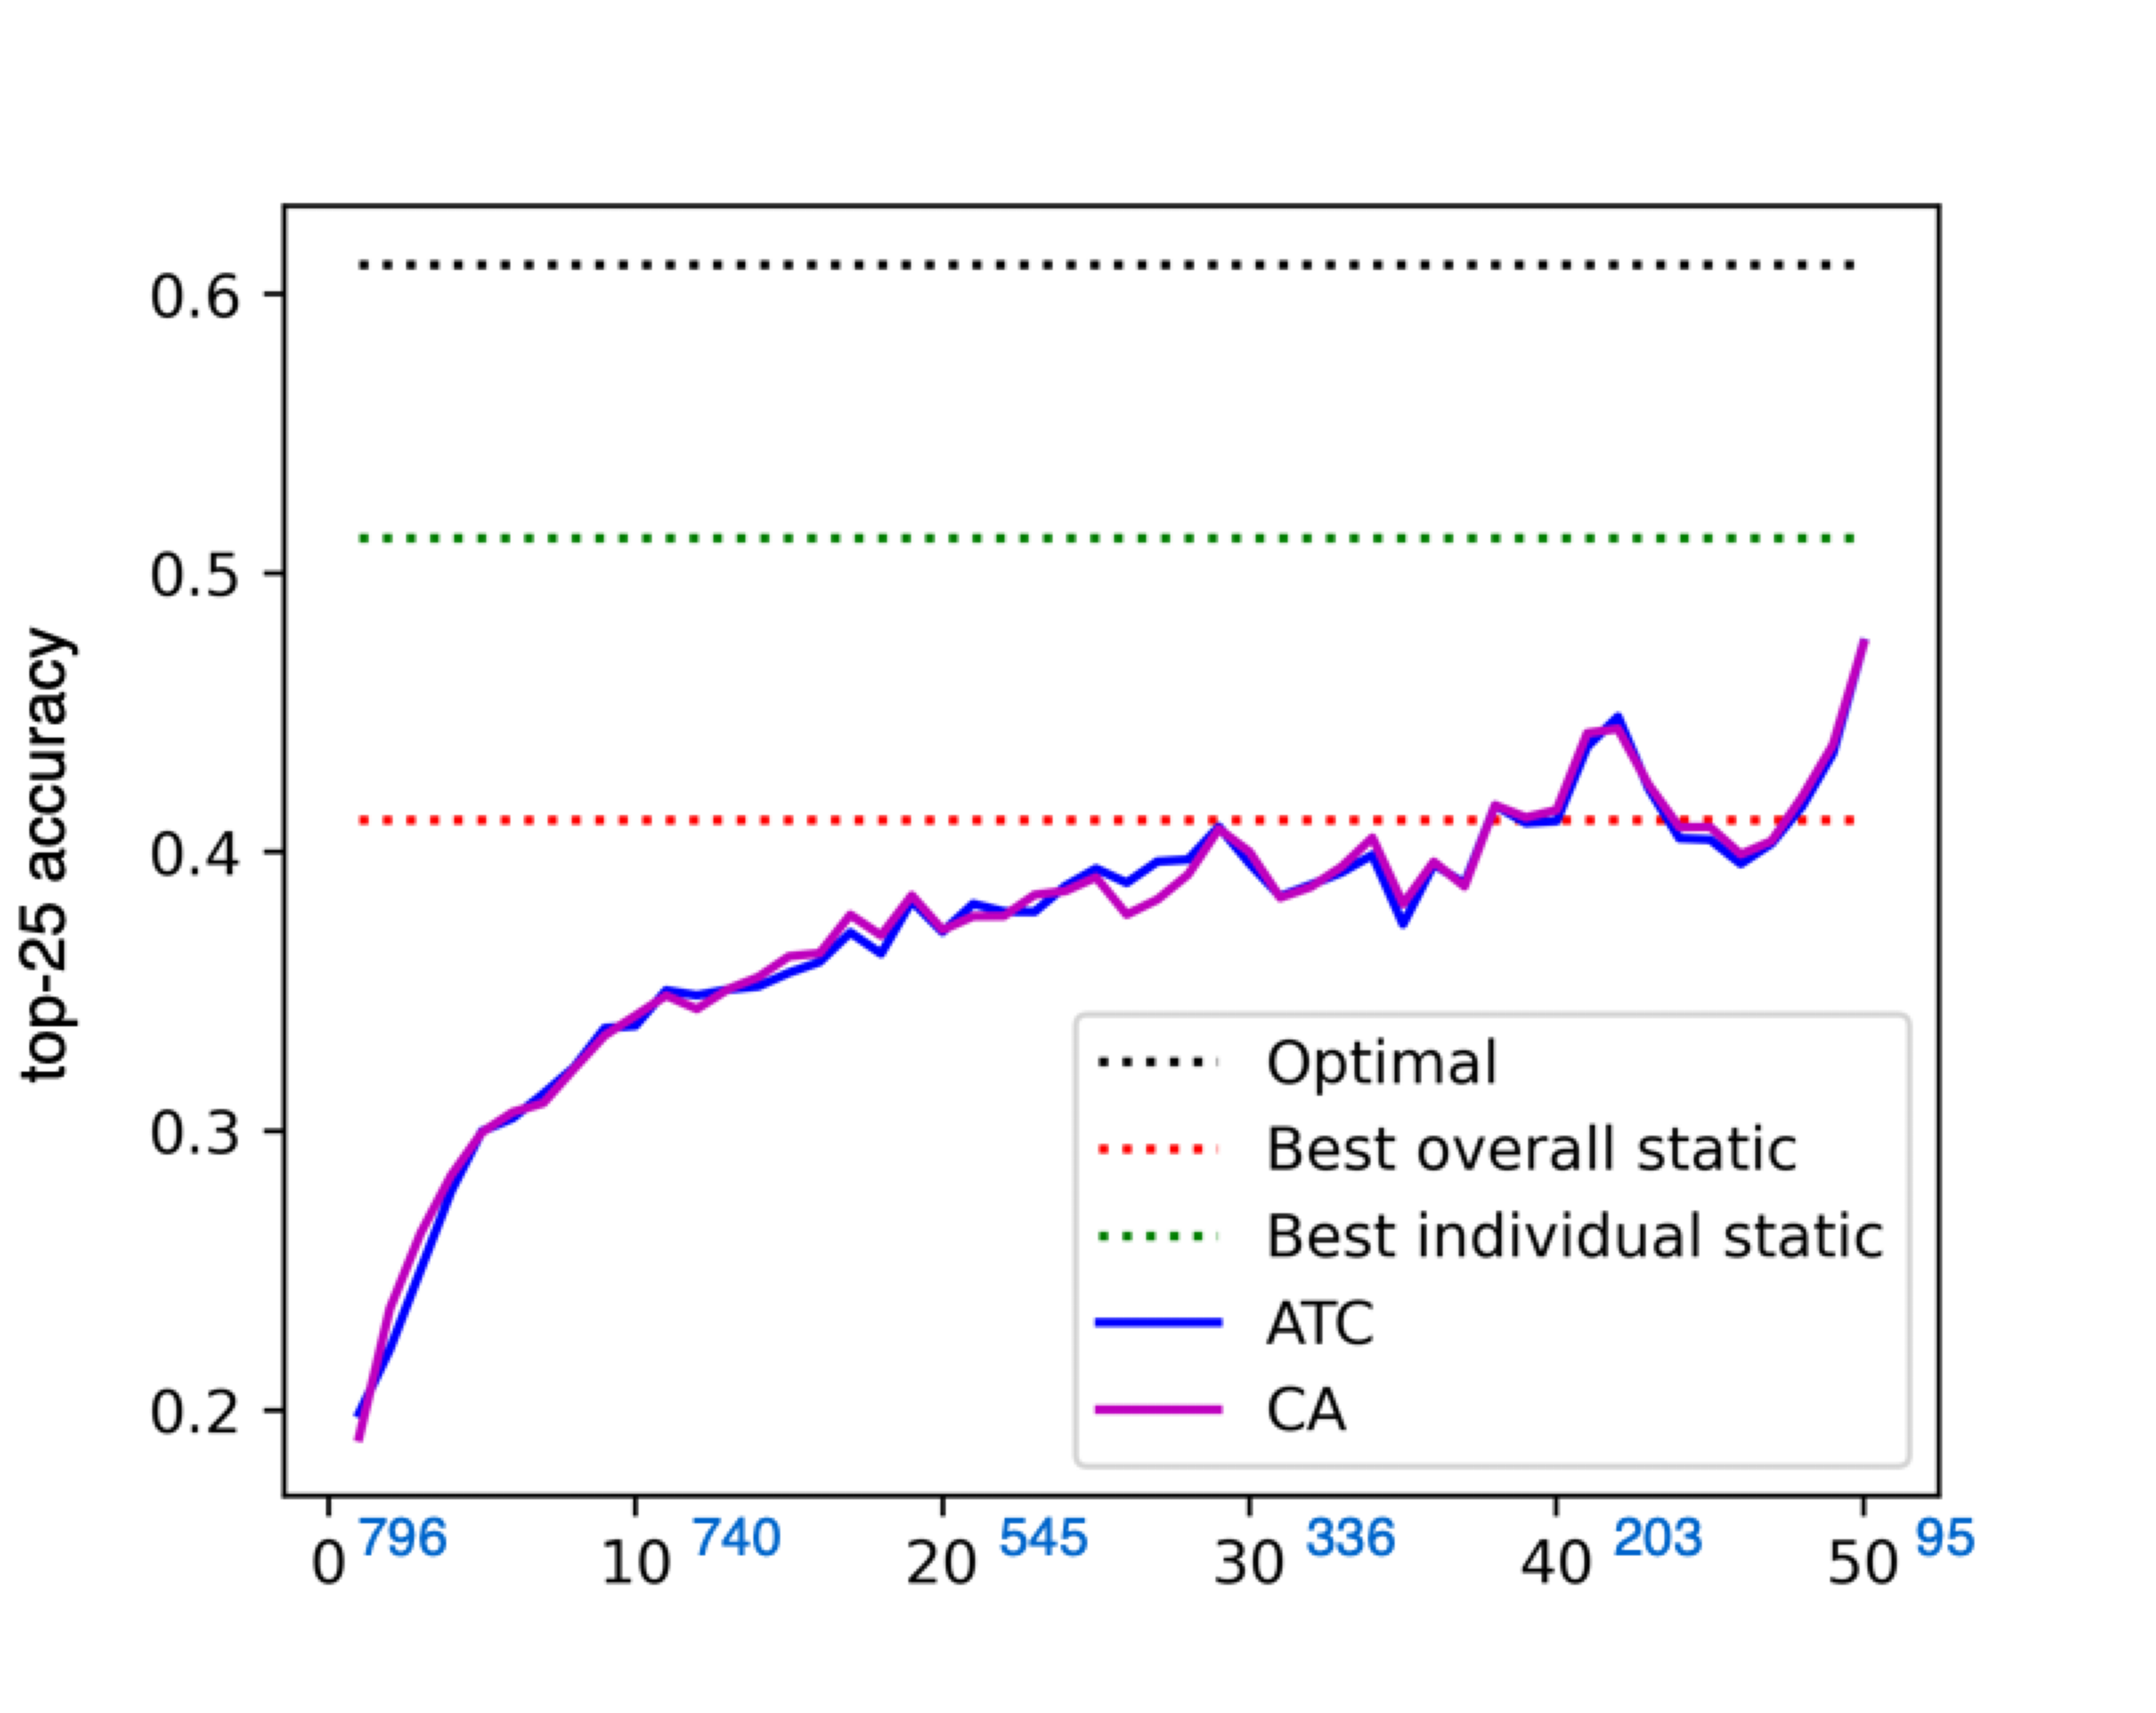}
    \caption{Top-$25$ accuracy comparison of adaptive and static approaches.}
    \label{fig:top25}
\end{figure}
\begin{figure}
    \centering
    \includegraphics[width=0.48\textwidth]{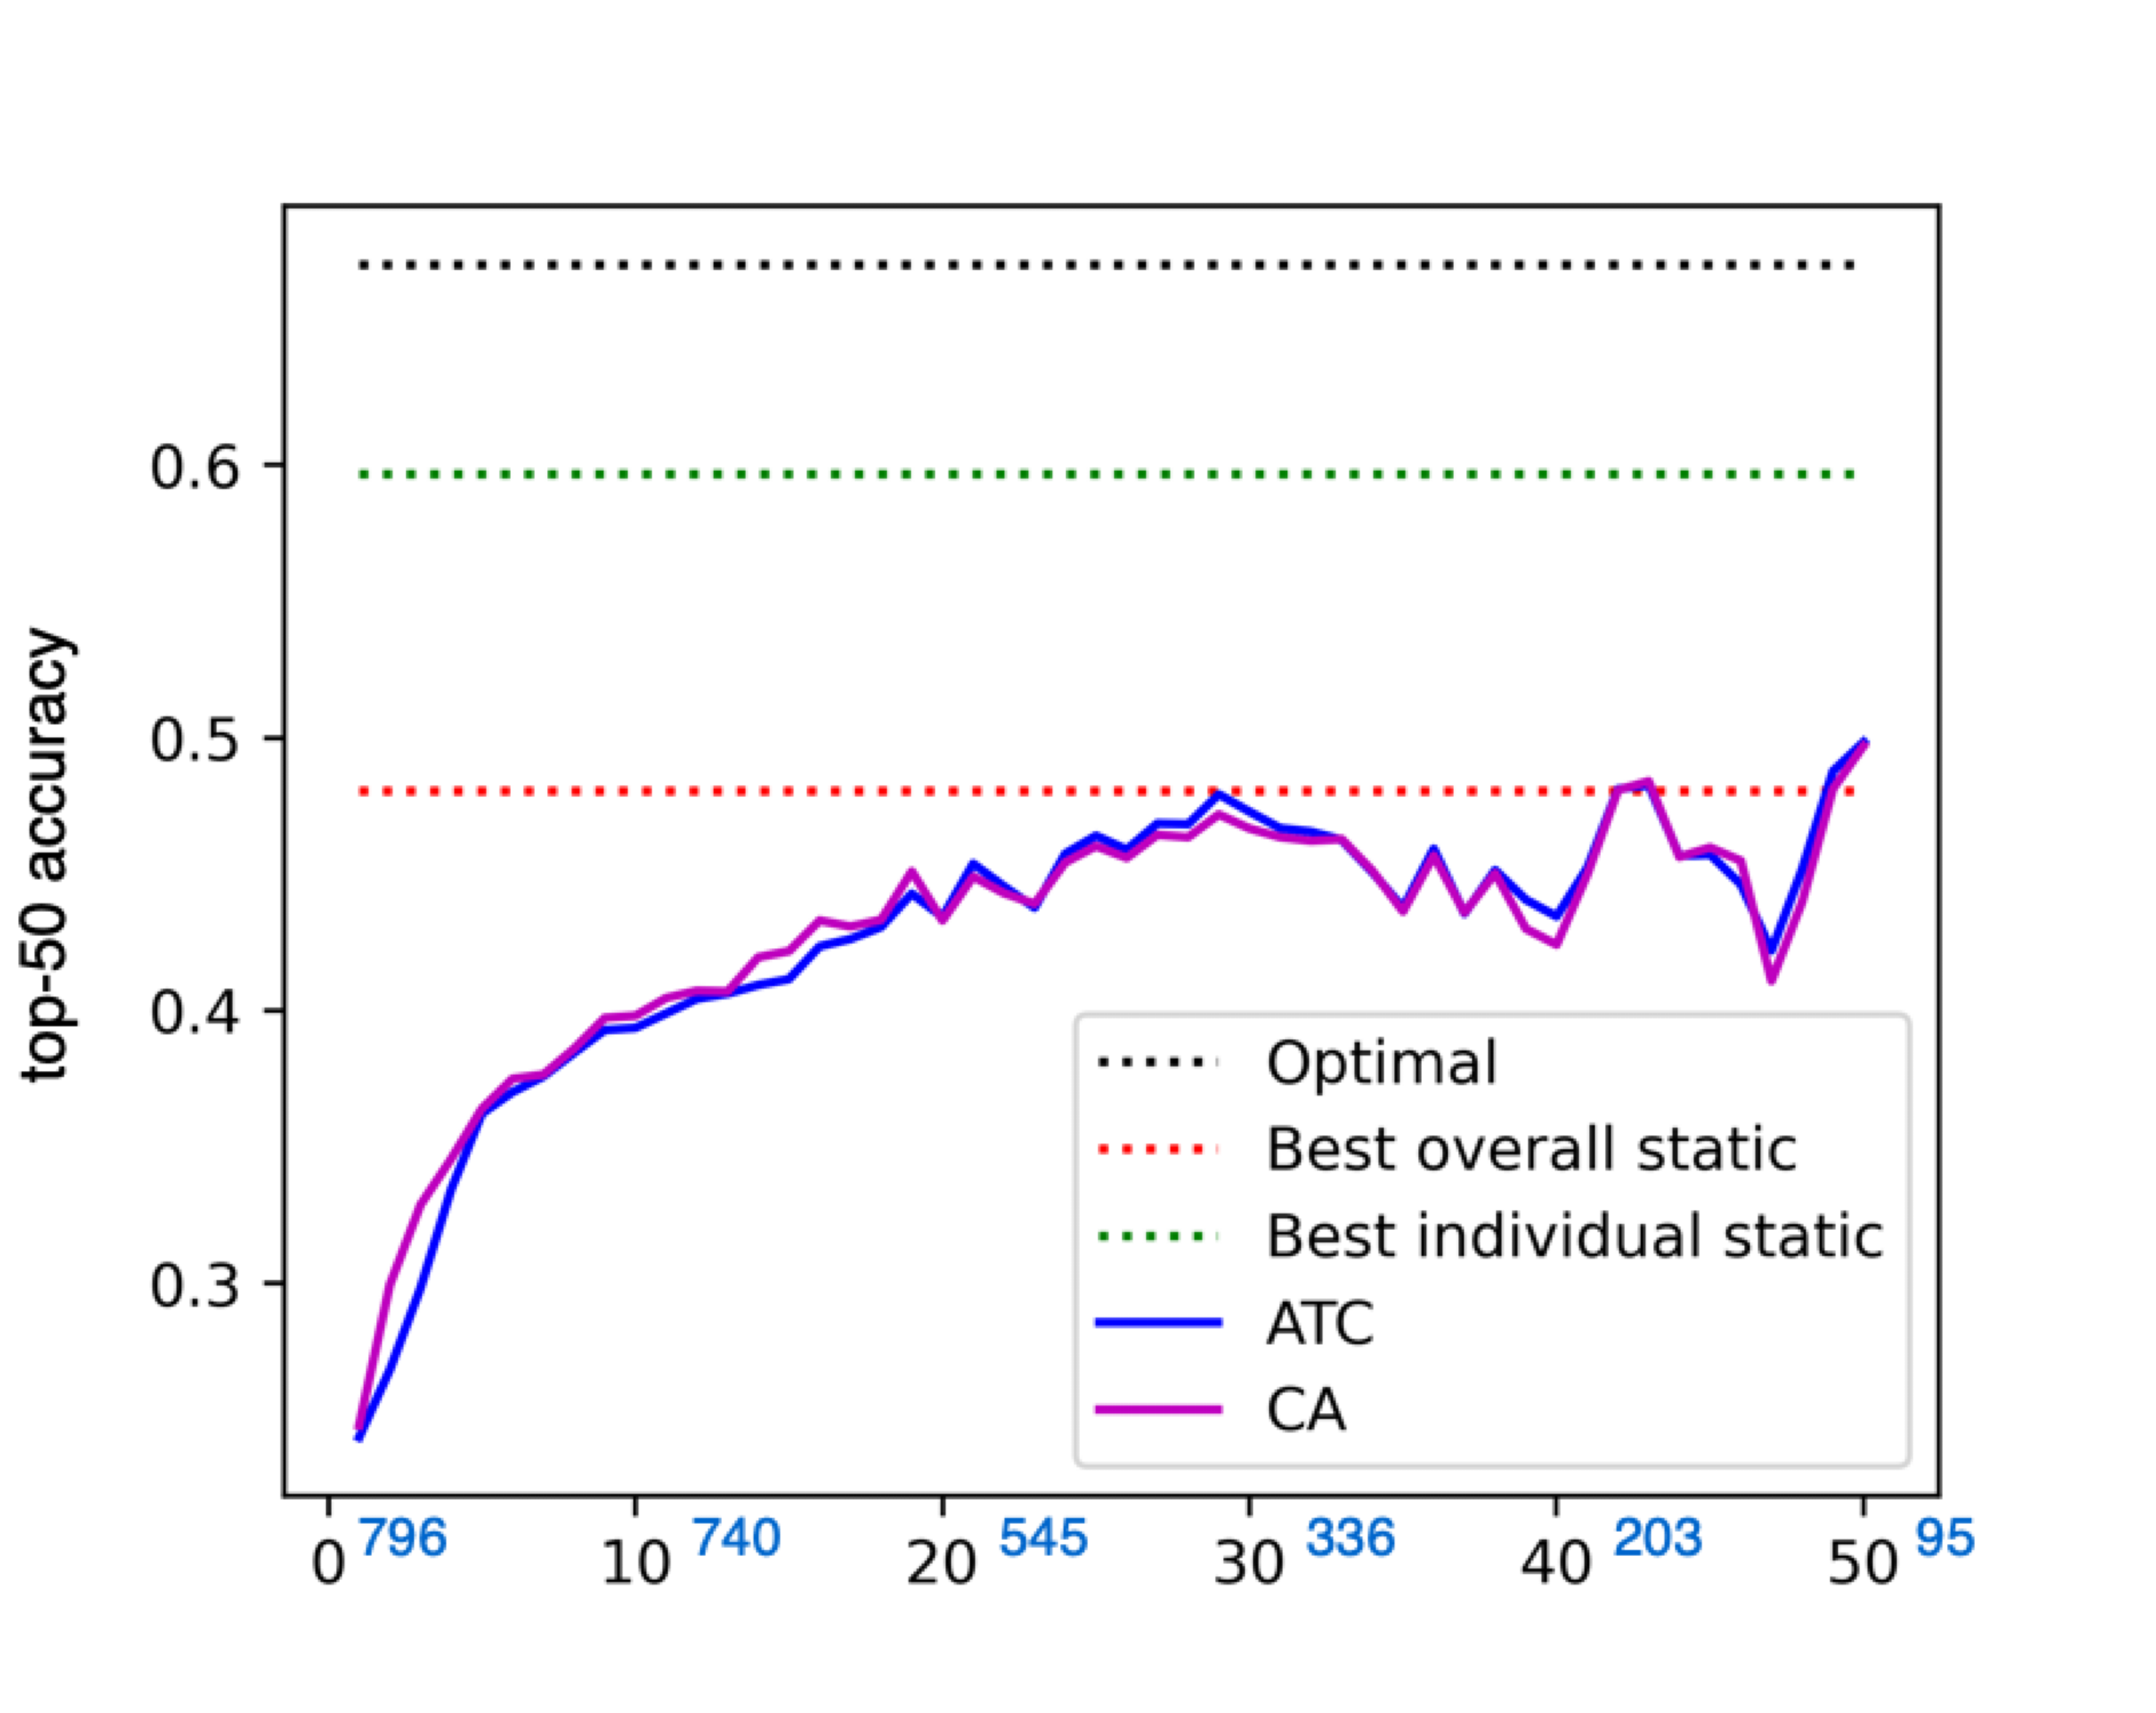}
    \caption{Top-$50$ accuracy comparison of adaptive and static approaches.}
    \label{fig:top50}
\end{figure}
